# Supplementary material for: UAV4D: Dynamic Neural Rendering of Human-Centric UAV Imagery using Gaussian Splatting
Source: arXiv:2506.05011 source file (2025-06-05)
Supplement: Supplementary file 1 [file breakdown_manipal_human.tex]

% \begin{table}[h]
%     \centering
%     \caption{\textbf{Breakdown results on the Manipal-UAV dataset} \cite{akshatha2023manipal}, focusing on \textbf{human-only} regions. Red, orange, and yellow indicate the first, second, and third best performing algorithms for each metric.}
%     \begin{adjustbox}{width=0.99\linewidth,center}
%     \begin{tabular}{l|cc|cc|cc|cc|cc}
%     \toprule
%     \multirow{2}{*}{Method }&\multicolumn{2}{c|}{40\_GND\_P1}&\multicolumn{2}{c|}{40\_VGT\_P1}&\multicolumn{2}{c|}{50\_GND\_P1}&\multicolumn{2}{c|}{50\_RD\_P1}&\multicolumn{2}{c}{Mean}\\
%     & PSNR \(\uparrow\)  & SSIM \(\uparrow\)  & PSNR \(\uparrow\)  & SSIM \(\uparrow\) & PSNR \(\uparrow\)  & SSIM \(\uparrow\)  & PSNR \(\uparrow\)  & SSIM \(\uparrow\)  & PSNR \(\uparrow\)  & SSIM \(\uparrow\)  \\
%     \midrule
% TK-Planes \cite{maxey2024tk}   & 20.52 &  \cellcolor{tabthird}0.838 & \cellcolor{tabsecond}15.79 & 0.577 & 19.11 & 0.822 & 18.11 & 0.769 & 18.38 & 0.752 \\
% 3DGS \cite{kerbl20233d}        & 19.35 & 0.816 & 15.45 & 0.587 & 18.55 & 0.798 &  \cellcolor{tabthird}18.60 & \cellcolor{tabsecond}0.791 & 17.99 & 0.748 \\
% 4DGS \cite{yang2024deformable} & \cellcolor{tabsecond}21.41 & \cellcolor{tabsecond}0.845 &  \cellcolor{tabfirst}15.83 &  \cellcolor{tabfirst}0.603 & \cellcolor{tabsecond}20.98 & \cellcolor{tabsecond}0.850 & \cellcolor{tabsecond}18.68 &  \cellcolor{tabthird}0.783 & \cellcolor{tabsecond}19.23 & \cellcolor{tabsecond}0.770 \\
% DeformableGS \cite{wu20244d}   &  \cellcolor{tabthird}20.66 & 0.837 &  \cellcolor{tabthird}15.64 & \cellcolor{tabsecond}0.597 &  \cellcolor{tabthird}20.27 &  \cellcolor{tabthird}0.843 & 18.05 & 0.771 &  \cellcolor{tabthird}18.65 &  \cellcolor{tabthird}0.762 \\
% Our Method                     &  \cellcolor{tabfirst}21.92 &  \cellcolor{tabfirst}0.880 & 15.61 &  \cellcolor{tabthird}0.594 &  \cellcolor{tabfirst}21.24 &  \cellcolor{tabfirst}0.872 &  \cellcolor{tabfirst}18.76 &  \cellcolor{tabfirst}0.792 &  \cellcolor{tabfirst}19.38 &  \cellcolor{tabfirst}0.784 \\
%     \bottomrule
%     \end{tabular}
%     \end{adjustbox}
%     \label{tab:breakdown_manipal_human}
% \end{table}
