# Supplementary material for: UAV4D: Dynamic Neural Rendering of Human-Centric UAV Imagery using Gaussian Splatting
Source: arXiv:2506.05011 source file (2025-06-05)
Supplement: Supplementary file 2 [file breakdown_okutama_human.tex]

% \begin{table}[h]
%     \centering
%     \caption{\textbf{Breakdown results on the Okutama-Action dataset} \cite{barekatain2017okutama}, focusing on \textbf{human-only} regions. Red, orange, and yellow indicate the first, second, and third best performing algorithms for each metric.}
%     \begin{adjustbox}{width=0.85\linewidth,center}
%     \begin{tabular}{l|cc|cc|cc|cc|cc}
%     \toprule
%     \multirow{2}{*}{Method }&\multicolumn{2}{c|}{1\_2\_2}&\multicolumn{2}{c|}{1\_2\_6}&\multicolumn{2}{c|}{1\_2\_8}&\multicolumn{2}{c|}{1\_2\_9}&\multicolumn{2}{c}{Mean}\\
%     & PSNR \(\uparrow\)  & SSIM \(\uparrow\)  & PSNR \(\uparrow\)  & SSIM \(\uparrow\) & PSNR \(\uparrow\)  & SSIM \(\uparrow\)  & PSNR \(\uparrow\)  & SSIM \(\uparrow\)  & PSNR \(\uparrow\)  & SSIM \(\uparrow\)  \\
%     \midrule
% TK-Planes \cite{maxey2024tk}   & 18.94 & 0.635 & 20.91 & 0.671 & 18.34 & 0.667 &  \cellcolor{tabfirst}18.39 &  \cellcolor{tabfirst}0.550 & \cellcolor{tabsecond}19.14 &  \cellcolor{tabthird}0.631 \\
% 3DGS \cite{kerbl20233d}        &  \cellcolor{tabfirst}19.97 &  \cellcolor{tabfirst}0.714 &  \cellcolor{tabthird}21.05 &  \cellcolor{tabthird}0.701 &  \cellcolor{tabthird}18.76 &  \cellcolor{tabthird}0.694 & 16.50 & 0.513 &  \cellcolor{tabthird}19.07 & \cellcolor{tabsecond}0.656 \\
% 4DGS \cite{yang2024deformable} & 15.80 & 0.504 &  \cellcolor{tabfirst}22.28 &  \cellcolor{tabfirst}0.735 & \cellcolor{tabsecond}19.65 & \cellcolor{tabsecond}0.725 & 14.99 & 0.446 & 18.18 & 0.602 \\
% DeformableGS \cite{wu20244d}   & \cellcolor{tabsecond}19.52 & \cellcolor{tabsecond}0.702 & 13.43 & 0.505 & 15.51 & 0.565 &  \cellcolor{tabthird}16.86 &  \cellcolor{tabthird}0.514 & 16.33 & 0.571 \\
% Our Method                     &  \cellcolor{tabthird}19.01 &  \cellcolor{tabthird}0.667 & \cellcolor{tabsecond}21.07 & \cellcolor{tabsecond}0.704 &  \cellcolor{tabfirst}19.70 &  \cellcolor{tabfirst}0.734 & \cellcolor{tabsecond}18.19 & \cellcolor{tabsecond}0.549 &  \cellcolor{tabfirst}19.49 &  \cellcolor{tabfirst}0.664 \\ 
%     \bottomrule
%     \end{tabular}
%     \end{adjustbox}
%     \label{tab:breakdown_okutama_human}
% \end{table}
